# Supplementary material for: When is more search useful? An Empirical Study of Search Utility in Quality-Aware Decoding for Machine Translation
Source: arXiv:2610.32679 source file (2026-11-03)
Supplement: Supplementary file 1 [file appendix.tex]

\appendix
